# Supplementary material for: Efficient model compression with Random Operation Access Specific Tile (ROAST) hashing
Source: arXiv:2207.10702 source file (2022-07-21)
Supplement: Supplementary file 2 [file appendix_theory.tex]

In this paper we introduce a generic model compression technique that disentangles functional expression from memory usage in a system-friendly manner. It is different from ROBE-Z in the sense that ROBE-Z only performs embedding compression. Also, it is different from the hashnet in the sense that hashnet only applies matrix compression and it is memory inefficient. Random-Offset-Block-Sketches is a generalized model compression which performs operation specific system-friendly lookup and maintains a single memory across the model. This raises some interesting theoretical questions

\subsection{Backward pass for model sharing weights across different components} \label{sec:gradexp}
A general function sharing a weight, say $x$ across different components can be written as , $f(x, g(x))$ The interpretation is that x was used in g(.) and then again used ahead in f. (In case of MLP, we can think of x being used in multiple layers)

Let $f(g_1, g_2)$ where both $g_1$ and $g_2$ are functions of $x$. 

\begin{align}
    \frac{\partial f(g_1, g_2)}{\partial x} = \frac{\partial f(g_1, g_2)}{\partial g_1} * \frac{\partial g_1}{\partial x} +  \frac{\partial f(g_1, g_2)}{\partial g_2}  * \frac{\partial g_2}{\partial x}
\end{align}

$g_1 = x$ and $g_2 = g(x)$

\begin{align}
    \frac{\partial f(g_1, g_2)}{\partial x} = \frac{\partial f(x, g(y))}{\partial x} |_{y=x} +  \frac{\partial f(y, g(x))}{\partial g(x)}  * \frac{\partial g(x)}{\partial x}|_{y=x}
\end{align}

\begin{align}
    \frac{\partial f(g_1, g_2)}{\partial x} = \frac{\partial f(x, g(y))}{\partial x}|_{y=x} +  \frac{\partial f(y, g(x))}{\partial x} |_{y=x}
\end{align}
Renaming,
\begin{align}
    \frac{\partial f(x, g(x))}{\partial x} = \frac{\partial f(z, g(y))}{\partial z}|_{y=x, z=x} +  \frac{\partial f(z, g(y))}{\partial y} |_{y=x, z=x}
\end{align}
Thus, we can essentially consider each place where x appears as new variables and then gradient w.r.t x is just summation of partial derivatives of the function w.r.t these new variables. Thus, it is easy to implement this in the backward pass. In order to make sure that the memory utilization in backward pass is not of the order of the recovered model size, we do not use the auto-differentiation of tensorflow/pytorch. We implement our own backward pass and it can be found in the code.

\subsection{Global feature hashing vs local feature hashing.}
In this section, we highlight the benefit of sharing the weights across the entire model as opposed to local sharing as was suggested in hashnet. We will show theory on a case which will illustrate the benefit without going into a very generic case.

\textbf{Setting:}
We will use the feature hashing - popular dimensionality reduction approach. Consider a vectors $x, y \in R^{n = n_1 +  n_2}$. We will compare the two settings. Let $x = [a, b]$ where $a \in R^{n_1}$ and $b \in R^{n_2}$. Let $y = [c, d]$ where $c \in R^{n_1}, d\in R^{n_2}$ . We will hash each vector into a vector of size $m$.

\begin{itemize}
    \item \textbf{Local weight-sharing} (as suggested by hashnet \cite{hashtrick}) : In this case we perform a local hashing into separate memory banks. So a and c are hashed into memory of size $\frac{n_1}{(n_1+n_2)}  m$ and b and d are hashed into separate memory of size $\frac{n_2}{(n_1+n_2)} m$
    \item \textbf{Global weight-sharing} (as suggested in this paper) we hash the entire vector x and y in the memory of size m.
 \end{itemize}
 
 You can think of a and b to be different flattened parameter vectors of two matrices. Generally the matrices are initialized specific to its size. Specifically, if the matrix corresponding to a is large, it will initialized with smaller values. To capture this difference, we will make some assumption on the norms of a ,b and c,d. Specifically, \todo{$||a||=||b||=||c||=||d||$}

 \textbf{Expectation}
 The suffix L refers to local hashing and G refers to global hashing.
 
 \begin{align}
     \mathbb{E}_G (\hat{\ip{x}{y}}) =  \ip{x}{y}
 \end{align}
 
 \begin{align}
     \mathbb{E}_L (\hat{\ip{x}{y}}) =  \mathbb{E}_G (\hat{\ip{a}{c}}) + \mathbb{E}_G (\hat{\ip{b}{d}}) =  \ip{x}{y}
 \end{align}

\textbf{Variance}
\begin{align}
    \mathbb{V}_G (\hat{\ip{x}{y}}) = \frac{1}{m} ( \sum_{i\neq j} (x_i^2 y_j^2 + x_i y_i x_j y_j ))
\end{align}

\begin{align}
    \mathbb{V}_G (\hat{\ip{a}{c}}) = \frac{n_1 + n_2}{n_1} \frac{1}{m} ( \sum_{i\neq j} (a_i^2 c_j^2 + a_i c_i a_j c_j ))
\end{align}

\begin{align}
    \mathbb{V}_G (\hat{\ip{b}{d}}) = \frac{n_1 + n_2}{n_2} \frac{1}{m} ( \sum_{i\neq j} (b_i^2 d_j^2 + b_i d_i b_j d_j ))
\end{align}

\begin{align}
    \mathbb{V}_G (\hat{\ip{x}{y}}) = \frac{1}{m} ( ||x||_2^2 ||y||_2^2 + \ip{x}{y}^2 - 2 ||x \circ y||_2^2)
\end{align}

\begin{align}
    \mathbb{V}_G (\hat{\ip{a}{c}}) = \frac{n_1 + n_2}{n_1} \frac{1}{m} ( ||a||_2^2 ||c||_2^2 + \ip{a}{c}^2 - 2 ||a \circ c||_2^2)
\end{align}

\begin{align}
    \mathbb{V}_G (\hat{\ip{b}{d}}) = \frac{n_1 + n_2}{n_2} \frac{1}{m} ( ||b||_2^2 ||d||_2^2 + \ip{b}{d}^2 - 2 ||b \circ d||_2^2)
\end{align}

\begin{align}
    \mathbb{V}_L(\hat{\ip{x}{y}}) = \mathbb{V}_G (\hat{\ip{a}{c}}) + \mathbb{V}_G (\hat{\ip{b}{d}})
\end{align}

Note that,

\begin{align}
\mathbb{V}_G (\hat{\ip{x}{y}}) = \frac{1}{m} (( \sum_{i\neq j} (a_i^2 c_j^2 + a_i c_i a_j c_j ) + \sum_{i\neq j} (b_i^2 d_j^2 + b_i d_i b_j d_j ) +  \sum (a_i^2 d_j^2 + (b_i^2 c_j^2) + a_i c_i b_j d_j ))
\end{align}

Let $f_1 = \frac{n_1}{n_1 + n_2}$ $f_2 = \frac{n_2}{n_1 + n_2}$

\begin{align}
\mathbb{V}_G (\hat{\ip{x}{y}}) = f_1 V_1  + f_2 V_2 + \frac{1}{m} (\sum (a_i^2 d_j^2 + (b_i^2 c_j^2) + a_i c_i b_j d_j ))
\end{align}

\begin{align}
\mathbb{V}_G (\hat{\ip{x}{y}}) = f_1 V_1  + f_2 V_2 + \frac{1}{m} (\sum (a_i^2 d_j^2 + (b_i^2 c_j^2) + a_i c_i b_j d_j ))
\end{align}

% \begin{equation}
%     \ip{x}{y} = \ip{a}{c} + \ip{b}{d}
% \end{equation}

% \begin{equation}
%     \ip{x}{y}^2 = \ip{a}{c}^2 + \ip{b}{d}^2  + 2 \ip{a}{c} \ip{b}{d} \leq 3 (\ip{a}{c}^2 + \ip{b}{d}^2)
% \end{equation}

% \begin{equation}
%     || x \circ y||_2^2 = || a \circ c||_2^2 + || b \circ d ||_2^2
% \end{equation}

% \begin{equation}
%     ||x||_2^2 ||y||_2^2  =||a||_2^2 ||c||_2^2 + ||b||_2^2 ||d||_2^2 + ||b||_2^2 ||c||_2^2 + ||a||_2^2 ||d||_2^2
% \end{equation}

\subsection{Global vs local feature hashing : The role of dependence in hashing quality}
In this section , we will show why global-weight-sharing gives better quality in feature hashing. Let us first define global vs local weight sharing in context of feature hashing. Consider we have a parameter-vector x. Let x can be written as a concatenation of k vectors. For simplicity, we assume that each of these parts is of equal length. We will look at norm preservation under hashing. We know that if norms are approximately preserved then inner products are also preserved under hashing.

\begin{equation}
    x \in R^n, x_i \in R^{n/k}
\end{equation}

\begin{equation}
    x = [x_1, x_2, ... x_k]
\end{equation}

\textbf{Global Feature hashing} In this case the entire parameter vector x is hashed into the vector of size m. In the most generic form we can write the equation that with probability $(1-\delta)$, we can hash the vector x into vector of size $m$ such that the norm is within $\epsilon$ multiplicative error. 
\begin{equation}
    \mathbb{P}(|\hat{||x||^2} - ||x||^2| \leq ||x|| \epsilon) = (1 - \delta)
\end{equation}
where $\delta = \Phi(\epsilon, m)$ where $\Phi$ is a decreasing function w.r.t m and $\epsilon$. 

\textbf{Some comments on the function $\Phi$}
We know that this function is decreasing function w.r.t m $\epsilon$. Using chernoff bounds we can bound this function by 
\begin{equation}
    \Phi(\epsilon, m) \leq \mathcal{O} (\exp(- m \epsilon^2))
\end{equation}

\textbf{Local feature hashing} In this we will be hashing each of the $x_i$ into vector of size m/k. Norm preservation guarantee for each independent local hashing is same as that for global with smaller array size of $m/k$
For each i,
\begin{equation}
    \mathbb{P}(|\hat{||x_i||^2} - ||x_i||^2| \leq ||x_i|| \epsilon_i) = (1 - \delta_i)
\end{equation}

where $\delta_i = \Phi(m/k, \epsilon_i)$ where $\Phi$ is the same function. We will show that the failure probability is much larger in case of local feature hashing due to independent hashing. In order to ensure that 
$|\hat{||x||^2} - ||x||^2| \leq ||x|| \epsilon)$ we need to ensure that 

\begin{equation}
    |\hat{||x||^2} - ||x||^2| 
    \leq \sum_{i} (|\hat{||x_i||^2} - ||x_i||^2|) \leq \epsilon ||x||^2
\end{equation}

\begin{equation}
    \sum_{i} (\epsilon_i ||x_i||^2) \leq \epsilon \||x||^2
\end{equation}
{\color{red} This is to be ensured for any particular  $x \in R^n$.
The only way to ensure this is to ensure that for all i, we have 
\begin{equation}
(|\hat{||x_i||^2} - ||x_i||^2|) \leq \epsilon ||x_i||_2
\end{equation} }
For each of this event the probability of success is $(1-\Phi(m/k, \epsilon))$. Thus total probability of success is $(1-\Phi(m/k, \epsilon))^k$

\subsection{Global vs Local Variance}

\begin{equation}
\mathbb{V}_G (\hat{\ip{x}{y}}) = \sum_i (f_i V_i) + \frac{1}{m} (\sum_{i,j,i\neq j} (||x_i||^2 ||y_j||^2)) + \ip{x_i}{y_i} \ip{x_j}{y_j}
\end{equation}

\begin{equation}
\mathbb{V}_L (\hat{\ip{x}{y}}) = \sum_i (V_i)
\end{equation}

where 
\begin{equation}
    V_k = \frac{1}{f_i} \frac{1}{m} (\sum_{i\neq j} a_i^2 b_j^2  + \sum_{i \neq j} a_i b_i a_j b_j) \textrm{ where } x_k = [a_1, a_2 ... a_n] \textrm{ and } y_k = [b_1, b_2 ... b_n]
\end{equation}
\begin{equation}
    \sum_i f_i = 1
\end{equation}
